# Supplementary material for: Machine Reading Comprehension using Case-based Reasoning
Source: arXiv:2305.14815 source file (2023-12-05)
Supplement: Supplementary file 1 [file table_lexical_diversity_appendix.tex]

\begin{table*}[h]
\small
\centering

\begin{tabular}{ccccccccccccccccc}
\toprule
\bf Threshold  & \multicolumn{8}{c}{\textbf{Lexical Diversity Scores per Bucket and #Questions(C)}}  \\
% \cline{3-6}
& & 1 & C & 2 & C & 3 & C & 4 & C & 5 & C  & 6 & C & 7&C & 8&C \\
\midrule 
$0.0$ & $19.77$ & 1365 & $39.64$ &2024 &$59.00$ & 1555&$81.28$ &1087 &$111.07$ & 540&$149.66$ & 189&$216.75$ & 75&$329.03$ & 31\\
\bottomrule
\end{tabular}
\caption{Performance on extractive QA datasets. }
\label{tab:lexical_div_appendix}
\end{table*}
